# Supplementary material for: Metabolism, information, and viability in a simulated physically-plausible protocell
Source: arXiv:2405.04654 source file (2024-05-07)
Supplement: Supplementary file 1 [file Appendix.tex]

\appendix
% \section{Strands used in simulations}

%The DNA strands used for simulations are constructed by combining the following six substrands:
%\begin{align}
% %    \textrm{substrand 1:} \,\,\,\,\,\,      &\textrm{5'-AGA-3'}\label{eq:sub1}\\
%                                             &\textrm{3'-TCT-5'}\nonumber\\
% %    \textrm{substrand 2:} \,\,\,\,\,\,      &\textrm{5'-AAA-3'}\\
%                                             &\textrm{3'-TTT-5'}\nonumber\\
% %    \textrm{substrand 3:} \,\,\,\,\,\,      &\textrm{5'-AGA-3'}\\
%                                             &\textrm{3'-TTT-5'}\nonumber\\
% %    \textrm{substrand 4:} \,\,\,\,\,\,      &\textrm{5'-AGA-3'}\\
%                                             &\textrm{3'-TAT-5'}\nonumber\\
% %    \textrm{substrand 5:} \,\,\,\,\,\,      &\textrm{5'-A8oxoGA-3'}\\
%                                             &\textrm{3'-TCT-5'}\nonumber\\
% %    \textrm{substrand 6:} \,\,\,\,\,\,      &\textrm{5'-AAA-3'}\label{eq:sub6}\\
%                                             &\textrm{3'-TT-5'}\nonumber
%\end{align}

\begin{table}[H]
\footnotesize
    \begin{tabular}{|l|l|}
        \hline
        Strand & \multicolumn{1}{|p{1.8cm}|}{\centering Substrand\\ sequence} \\ \hline
\rowcolor{p} 1 & 1  1  6  1  1  5 \\
\rowcolor{p} 2 & 1  1  6  1  2  5 \\
\rowcolor{p} 3 & 1  1  6  1  3  5 \\
\rowcolor{p} 4 & 1  1  6  1  4  5 \\
\rowcolor{p} 5 & 1  1  6  1  5  1 \\
\rowcolor{p} 6 & 1  1  6  1  5  2 \\
\rowcolor{b} 7 & 1  1  6  2  1  5 \\
\rowcolor{b} 8 & 1  1  6  2  2  5 \\
\rowcolor{b} 9 & 1  1  6  2  5  1 \\
\rowcolor{b} 10 & 1  1  6  2  5  2 \\
\rowcolor{b} 11 & 1  1  6  5  1  1 \\
\rowcolor{b} 12 & 1  1  6  5  1  2 \\
\rowcolor{g} 13 & 1  1  6  5  1  3 \\
\rowcolor{g} 14 & 1  1  6  5  1  4 \\
\rowcolor{b} 15 & 1  1  6  5  2  1 \\
\rowcolor{b} 16 & 1  1  6  5  2  2 \\
\rowcolor{p} 17 & 1  2  6  1  1  5 \\
\rowcolor{p} 18 & 1  2  6  1  2  5 \\
\rowcolor{p} 19 & 1  2  6  1  3  5 \\
\rowcolor{p} 20 & 1  2  6  1  4  5 \\
\rowcolor{p} 21 & 1  2  6  1  5  1 \\
\rowcolor{p} 22 & 1  2  6  1  5  2 \\
\rowcolor{b} 23 & 1  2  6  2  1  5 \\
\rowcolor{b} 24 & 1  2  6  2  2  5 \\
\rowcolor{b} 25 & 1  2  6  2  5  1 \\
\rowcolor{b} 26 & 1  2  6  2  5  2 \\
\rowcolor{b} 27 & 1  2  6  5  1  1 \\
\rowcolor{b} 28 & 1  2  6  5  1  2 \\
\rowcolor{b} 29 & 1  2  6  5  1  3 \\
\rowcolor{b} 30 & 1  2  6  5  1  4 \\
\rowcolor{b} 31 & 1  2  6  5  2  1 \\
\rowcolor{b} 32 & 1  2  6  5  2  2 \\
\rowcolor{p} 33 & 1  3  6  1  1  5 \\
\rowcolor{p} 34 & 1  3  6  1  2  5 \\
\rowcolor{g} 35 & 1  3  6  1  3  5 \\
\rowcolor{r} 36 & 1  3  6  1  4  5 \\
\rowcolor{p} 37 & 1  3  6  1  5  1 \\
\rowcolor{p} 38 & 1  3  6  1  5  2 \\
\rowcolor{p} 39 & 1  3  6  2  1  5 \\
\rowcolor{p} 40 & 1  3  6  2  2  5 \\
\hline \end{tabular} \hspace{0.25cm} \begin{tabular}{|l|l|} \hline Strand & \multicolumn{1}{|p{1.8cm}|}{\centering Substrand\\ sequence} \\ \hline
\rowcolor{p} 41 & 1  3  6  2  5  1 \\
\rowcolor{p} 42 & 1  3  6  2  5  2 \\
\rowcolor{p} 43 & 1  3  6  5  1  1 \\
\rowcolor{p} 44 & 1  3  6  5  1  2 \\
\rowcolor{g} 45 & 1  3  6  5  1  3 \\
\rowcolor{r} 46 & 1  3  6  5  1  4 \\
\rowcolor{p} 47 & 1  3  6  5  2  1 \\
\rowcolor{p} 48 & 1  3  6  5  2  2 \\
\rowcolor{p} 49 & 1  4  6  1  1  5 \\
\rowcolor{p} 50 & 1  4  6  1  2  5 \\
\rowcolor{r} 51 & 1  4  6  1  3  5 \\
\rowcolor{p} 52 & 1  4  6  1  4  5 \\
\rowcolor{p} 53 & 1  4  6  1  5  1 \\
\rowcolor{p} 54 & 1  4  6  1  5  2 \\
\rowcolor{p} 55 & 1  4  6  2  1  5 \\
\rowcolor{p} 56 & 1  4  6  2  2  5 \\
\rowcolor{p} 57 & 1  4  6  2  5  1 \\
\rowcolor{p} 58 & 1  4  6  2  5  2 \\
\rowcolor{p} 59 & 1  4  6  5  1  1 \\
\rowcolor{p} 60 & 1  4  6  5  1  2 \\
\rowcolor{r} 61 & 1  4  6  5  1  3 \\
\rowcolor{p} 62 & 1  4  6  5  1  4 \\
\rowcolor{p} 63 & 1  4  6  5  2  1 \\
\rowcolor{p} 64 & 1  4  6  5  2  2 \\
\rowcolor{p} \textcolor{red}{65} & \textcolor{red}{1  5  6  1  1  1} \\
\rowcolor{p} \textcolor{red}{66} & \textcolor{red}{1  5  6  1  1  2} \\
\rowcolor{g} \textcolor{red}{67} & \textcolor{red}{1  5  6  1  1  3} \\
\rowcolor{g} \textcolor{red}{68} & \textcolor{red}{1  5  6  1  1  4} \\
\rowcolor{p} \textcolor{red}{69} & \textcolor{red}{1  5  6  1  2  1} \\
\rowcolor{p} \textcolor{red}{70} & \textcolor{red}{1  5  6  1  2  2} \\
\rowcolor{p} \textcolor{red}{71} & \textcolor{red}{1  5  6  1  3  1} \\
\rowcolor{g} \textcolor{red}{72} & \textcolor{red}{1  5  6  1  3  2} \\
\rowcolor{p} \textcolor{red}{73} & \textcolor{red}{1  5  6  1  4  1} \\
\rowcolor{g} \textcolor{red}{74} & \textcolor{red}{1  5  6  1  4  2} \\
\rowcolor{p} \textcolor{red}{75} & \textcolor{red}{1  5  6  2  1  1} \\
\rowcolor{p} \textcolor{red}{76} & \textcolor{red}{1  5  6  2  1  2} \\
\rowcolor{p} \textcolor{red}{77} & \textcolor{red}{1  5  6  2  1  3} \\
\rowcolor{p} \textcolor{red}{78} & \textcolor{red}{1  5  6  2  1  4} \\
\rowcolor{p} \textcolor{red}{79} & \textcolor{red}{1  5  6  2  2  1} \\
\rowcolor{p} \textcolor{red}{80} & \textcolor{red}{1  5  6  2  2  2} \\
\hline \end{tabular} \hspace{0.25cm} \begin{tabular}{|l|l|} \hline Strand & \multicolumn{1}{|p{1.8cm}|}{\centering Substrand\\ sequence} \\ \hline
\rowcolor{p} 81 & 2  1  6  1  1  5 \\
\rowcolor{p} 82 & 2  1  6  1  2  5 \\
\rowcolor{p} 83 & 2  1  6  1  3  5 \\
\rowcolor{p} 84 & 2  1  6  1  4  5 \\
\rowcolor{p} 85 & 2  1  6  1  5  1 \\
\rowcolor{p} 86 & 2  1  6  1  5  2 \\
\rowcolor{p} 87 & 2  1  6  2  1  5 \\
\rowcolor{b} 88 & 2  1  6  2  2  5 \\
\rowcolor{b} 89 & 2  1  6  2  5  1 \\
\rowcolor{b} 90 & 2  1  6  2  5  2 \\
\rowcolor{p} 91 & 2  1  6  5  1  1 \\
\rowcolor{p} 92 & 2  1  6  5  1  2 \\
\rowcolor{g} 93 & 2  1  6  5  1  3 \\
\rowcolor{g} 94 & 2  1  6  5  1  4 \\
\rowcolor{b} 95 & 2  1  6  5  2  1 \\
\rowcolor{b} 96 & 2  1  6  5  2  2 \\
\rowcolor{p} 97 & 2  2  6  1  1  5 \\
\rowcolor{p} 98 & 2  2  6  1  2  5 \\
\rowcolor{p} 99 & 2  2  6  1  3  5 \\
\rowcolor{p} 100 & 2  2  6  1  4  5 \\
\rowcolor{p} 101 & 2  2  6  1  5  1 \\
\rowcolor{p} 102 & 2  2  6  1  5  2 \\
\rowcolor{p} 103 & 2  2  6  2  1  5 \\
\rowcolor{p} 104 & 2  2  6  2  2  5 \\
\rowcolor{p} 105 & 2  2  6  2  5  1 \\
\rowcolor{p} 106 & 2  2  6  2  5  2 \\
\rowcolor{p} 107 & 2  2  6  5  1  1 \\
\rowcolor{p} 108 & 2  2  6  5  1  2 \\
\rowcolor{p} 109 & 2  2  6  5  1  3 \\
\rowcolor{p} 110 & 2  2  6  5  1  4 \\
\rowcolor{p} 111 & 2  2  6  5  2  1 \\
\rowcolor{p} 112 & 2  2  6  5  2  2 \\
\rowcolor{p} \textcolor{red}{113} & \textcolor{red}{2  5  6  1  1  1} \\
\rowcolor{p} \textcolor{red}{114} & \textcolor{red}{2  5  6  1  1  2} \\
\rowcolor{p} \textcolor{red}{115} & \textcolor{red}{2  5  6  1  1  3} \\
\rowcolor{p} \textcolor{red}{116} & \textcolor{red}{2  5  6  1  1  4} \\
\rowcolor{p} \textcolor{red}{117} & \textcolor{red}{2  5  6  1  2  1} \\
\rowcolor{p} \textcolor{red}{118} & \textcolor{red}{2  5  6  1  2  2} \\
\rowcolor{p} \textcolor{red}{119} & \textcolor{red}{2  5  6  1  3  1} \\
\rowcolor{p} \textcolor{red}{120} & \textcolor{red}{2  5  6  1  3  2} \\
\hline \end{tabular} \hspace{0.25cm} \begin{tabular}{|l|l|} \hline Strand & \multicolumn{1}{|p{1.8cm}|}{\centering Substrand\\ sequence} \\ \hline
\rowcolor{p} \textcolor{red}{121} & \textcolor{red}{2  5  6  1  4  1} \\
\rowcolor{p} \textcolor{red}{122} & \textcolor{red}{2  5  6  1  4  2} \\
\rowcolor{p} \textcolor{red}{123} & \textcolor{red}{2  5  6  2  1  1} \\
\rowcolor{p} \textcolor{red}{124} & \textcolor{red}{2  5  6  2  1  2} \\
\rowcolor{p} \textcolor{red}{125} & \textcolor{red}{2  5  6  2  1  3} \\
\rowcolor{p} \textcolor{red}{126} & \textcolor{red}{2  5  6  2  1  4} \\
\rowcolor{p} \textcolor{red}{127} & \textcolor{red}{2  5  6  2  2  1} \\
\rowcolor{p} \textcolor{red}{128} & \textcolor{red}{2  5  6  2  2  2} \\
\rowcolor{p} \textcolor{red}{129} & \textcolor{red}{5  1  6  1  1  1} \\
\rowcolor{p} \textcolor{red}{130} & \textcolor{red}{5  1  6  1  1  2} \\
\rowcolor{p} \textcolor{red}{131} & \textcolor{red}{5  1  6  1  1  3} \\
\rowcolor{p} \textcolor{red}{132} & \textcolor{red}{5  1  6  1  1  4} \\
\rowcolor{p} \textcolor{red}{133} & \textcolor{red}{5  1  6  1  2  1} \\
\rowcolor{p} \textcolor{red}{134} & \textcolor{red}{5  1  6  1  2  2} \\
\rowcolor{p} \textcolor{red}{135} & \textcolor{red}{5  1  6  1  3  1} \\
\rowcolor{p} \textcolor{red}{136} & \textcolor{red}{5  1  6  1  3  2} \\
\rowcolor{p} \textcolor{red}{137} & \textcolor{red}{5  1  6  1  4  1} \\
\rowcolor{p} \textcolor{red}{138} & \textcolor{red}{5  1  6  1  4  2} \\
\rowcolor{p} \textcolor{red}{139} & \textcolor{red}{5  1  6  2  1  1} \\
\rowcolor{p} \textcolor{red}{140} & \textcolor{red}{5  1  6  2  1  2} \\
\rowcolor{p} \textcolor{red}{141} & \textcolor{red}{5  1  6  2  1  3} \\
\rowcolor{p} \textcolor{red}{142} & \textcolor{red}{5  1  6  2  1  4} \\
\rowcolor{p} \textcolor{red}{143} & \textcolor{red}{5  1  6  2  2  1} \\
\rowcolor{p} \textcolor{red}{144} & \textcolor{red}{5  1  6  2  2  2} \\
\rowcolor{p} \textcolor{red}{145} & \textcolor{red}{5  2  6  1  1  1} \\
\rowcolor{p} \textcolor{red}{146} & \textcolor{red}{5  2  6  1  1  2} \\
\rowcolor{p} \textcolor{red}{147} & \textcolor{red}{5  2  6  1  1  3} \\
\rowcolor{p} \textcolor{red}{148} & \textcolor{red}{5  2  6  1  1  4} \\
\rowcolor{p} \textcolor{red}{149} & \textcolor{red}{5  2  6  1  2  1} \\
\rowcolor{p} \textcolor{red}{150} & \textcolor{red}{5  2  6  1  2  2} \\
\rowcolor{p} \textcolor{red}{151} & \textcolor{red}{5  2  6  1  3  1} \\
\rowcolor{p} \textcolor{red}{152} & \textcolor{red}{5  2  6  1  3  2} \\
\rowcolor{p} \textcolor{red}{153} & \textcolor{red}{5  2  6  1  4  1} \\
\rowcolor{p} \textcolor{red}{154} & \textcolor{red}{5  2  6  1  4  2} \\
\rowcolor{p} \textcolor{red}{155} & \textcolor{red}{5  2  6  2  1  1} \\
\rowcolor{p} \textcolor{red}{156} & \textcolor{red}{5  2  6  2  1  2} \\
\rowcolor{p} \textcolor{red}{157} & \textcolor{red}{5  2  6  2  1  3} \\
\rowcolor{p} \textcolor{red}{158} & \textcolor{red}{5  2  6  2  1  4} \\
\rowcolor{p} \textcolor{red}{159} & \textcolor{red}{5  2  6  2  2  1} \\
\rowcolor{p} \textcolor{red}{160} & \textcolor{red}{5  2  6  2  2  2} \\
\hline
    \end{tabular}
    \caption[Substrand sequences of simulated strands]{All strands used for simulations and their substrand sequences. The decomposition (nucleotide sequences) of substrands are shown in \autoref{eq:sub1}-\ref{eq:sub6}. Red cells contain strands which satisfies the condition for sufficiently fast CT and blue cells contain strands which satisfies the condition for sufficiently fast replication (see Section \ref{sec:FI}). Purple cells contain strands which satisfies both of the aforementioned conditions. Grey cells contain strands for which either the LIDA or CT simulation did not finish within the allotted time. Red text signifies a strand sequence containing an 8-oxo-G before the central bulge.}
% \end{longtable}
\label{tab:strands}
\end{table}
